# Supplementary material for: Dynamics of Reversible Plasticity in an Amorphous Solid
Source: arXiv:2512.17816 ancillary file (2025-12-19)
Supplement: Supplementary file 1 [file Supplemental_Materials.pdf]

# Supplemental Material for Dynamics of Reversible Plasticity in an Amorphous Solid

Zhicheng Wang and Nathan C. Keim

## SA. Methods

### *Sample preparation*

We mix the colloid suspensions proportionally to make a bidisperse suspension with roughly equal parts by number. It is then diluted with equal parts ethanol and water to about 2 w% and suspended with a vortex mixer. This carrier suspension is then pipetted and released as drops above the decane layer. Each drop sinks through the decane layer and releases its contents upon reaching the aqueous phase. Since alcohol has smaller surface tension than the decane-water interface, the droplet tends to expand rapidly across the decane-water interface, which spreads the particles. The interfacial tension is strong enough to confine the particles to the interface.

### *Interfacial shear channel setup*

A channel with length $L = 16.9$ mm and width $W = 2.38$ cm is cut in the top face of an aluminum rectangular prism. For a portion of the channel's length, the vertical cut extends all the way through this block, allowing light to pass from below. The water level is adjusted so that the interface is flush with the top of the aluminum block, creating a 2D channel with open boundaries at each end, so that particles can enter and exit freely.

A moving needle is set up along the long axis of the channel at the center, separating the channel in two, each forming a shear cell with length $L = 16.9$ mm and width $R = 1.08$ mm. The needle is in contact with both the fluid subphases and by proximity the particle monolayer which essentially creates a no-slip condition at its boundary. The needle is magnetized beforehand by rubbing against a permanent magnet.

We control the needle by the scheme of Qiao et al. [10]. The needle is trapped by a pair of permanent magnets placed above each end. By applying a magnetic field gradient along the direction of the needle, one applies a force on the needle. The field gradient is generated with a 500-turn magnetic coil, its magnetic axis being coincident with the needle axis, placed ~10 cm away. We operate in the small-gradient, small-displacement regime in which the force on the needle and the resulting displacement in the trap (with no adsorbed particles) are both linear in the electric current [10, 43].

The drive signal is passed to the coil by a power amplifier and a DAC device allowing arbitrary waveform generation. A typical test waveform consists of sinusoidal waveforms with variable amplitude and frequency, combined with pauses where the output is constant. The speed of the needle is always low so that $\mathrm{Re} < 1$ for the flow in the channel.

We image the central portion of the channel with a field of view of about 3 mm by 1 mm, including $> 35,000$ particles at area fraction $\sim 22\%$. The pixel size roughly corresponds to 0.78 $\mu$m by 0.78 $\mu$m. Particles are identified as centroids of dark spots against a brightly illuminated background. Particle identification and tracking can achieve precision of $< 0.1$ px which is $< 0.1$ $\mu$m. Trajectories are obtained with the trackpy Python package, using its channel-flow prediction capability.

The monolayer experiences the in-plane shear stress imposed by the needle, which would tend to create uniform shear and a linear displacement profile across the channel. However, particles are also coupled to the bulk flow of the oil and water that surrounds them, which is dominated by viscosity, but whose velocity profile is nonlinear because of the higher dimensionality [9, 44]. To verify that this coupling is weak and the shear of the monolayer is nearly uniform (i.e. high Boussinesq number), we check the displacement profile across the channel. Figure S1 plots each particle's displacement along the channel, as a function of its distance to the channel wall, showing a nearly linear relation on average. These data are taken at the highest frequency ($f = 0.124$ s$^{-1}$), at the instant of highest strain rate during a cycle (with $\dot{\gamma} = 0.023$ s$^{-1}$). This sample at maximum strain rate represents the worst case for all data in the paper, since deviations from a linear profile are dominated by viscous effects.

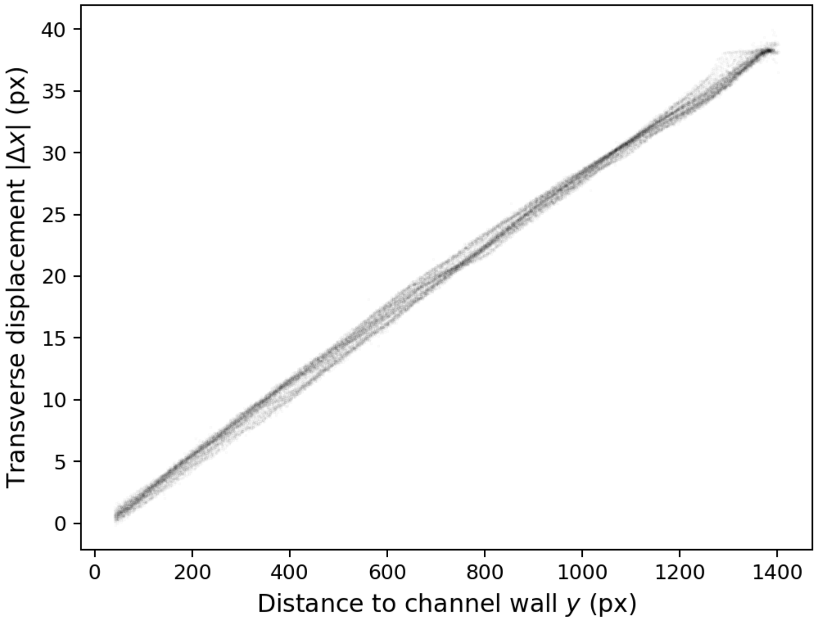


Figure S1: Particle displacement profile at the highest frequency $f = 0.124\ \mathrm{s}^{-1}$, showing the displacement of particles at $\gamma = \gamma_{\max}/2$ (highest average velocity during forward shear) compared to the start of the cycle. Each point represents one particle.

*Detecting rearrangements*

The response to a small shear strain ($< 1\%$) is nearly homogeneous. At higher shear strain ($< 10\%$) the fraction of non-affine displacements increases until they become system-sized, leading to a yielding transition in the monolayer. In most experiments reported the maximum strain is lower than this yielding transition point. In this case the rearrangements are localized. We use $D_{\min}$ to probe the non-affine displacements. Following conventions in literature, it is computed in a neighborhood including up to the second neighbor shell [4] and normalized with respect to the average nearest neighbor distance, $r_0$, corresponding to the location of the first peak in $g(r)$ [22].

*Preparatory protocols*

In the beginning of each experiment, we use a large shear strain ($> 10\%$) to reset the system. It leaves an imprint on the configuration and erases memories of previous strain amplitudes below yield. This is followed by a strain annealing protocol that ranges from 10% to 0.5% (Fig. S2). As shown previously [11], ring-down annealing drastically decreases the number of subsequent cycles needed to reach a steady state, so that the transient in an oscillatory experiment is one cycle. This allows repeatable measurements of rearrangements over multiple periods.

*Area Fraction Estimation*

We estimated the particle area fraction following the procedure in [17]. A low-pass filter of threshold 200 px is applied to the image. A binary filter is then applied to separate the particles from the background. We used a range of binary thresholds, so that no particle is omitted at the lowest threshold value, and disjoint particles do not overlap at the highest threshold value. A low value of 21.95% and a high value of 22.87% are recorded.

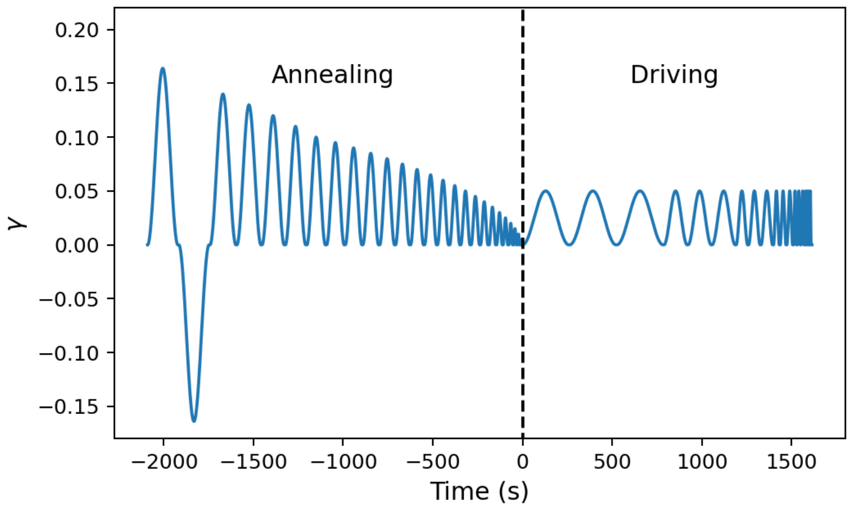


Figure S2: The driving waveform used in the experiment, showing the initial erasure, annealing protocol, and constant amplitude driving.

*Dissipation timescale*

Studies of charged polystyrene sulfate latex particles at a water-decane interface [40, 41] use the pair-correlation function of a very dilute monolayer (< 1% area fraction) to find an interaction energy between two particles of the form

$$\frac{U(r)}{k_B T} \sim \frac{a_{pp}}{r^3} \tag{S1}$$

where $a_{pp} \sim 1 \times 10^{-13}$ m$^3$. This earlier measurement is consistent with our own measurements of the particles in this study using a similar method [42], $a_{pp} \sim 5 \times 10^{-13}$ m$^{-3}$. However, since our measurement is noisier, we use the previously published value for this estimate. Using the typical interparticle distance $r_0 = 10$ $\mu$m from our experiments, we can estimate the interparticle force as

$$|F_{pp}| \sim \frac{k_B T \cdot a_{pp}}{r^4} = \frac{(4 \times 10^{-21}\ \text{J}) \cdot (10^{-13}\ \text{m}^3)}{(10^{-5}\ \text{m})^4} = 4 \times 10^{-14}\ \text{N}. \tag{S2}$$

We assume that at experimental shearing frequencies, well above the quasi-static limit, the rearranging motion of each particle is driven by a net force of order $F_{pp}$, which is balanced by Stokes drag on the particle. Both decane and water have a dynamic viscosity of around 0.9 mPa s. Then the velocity of the rearranging particle is estimated as

$$v = \frac{F_{pp}}{6\pi\mu R} = \frac{4 \times 10^{-14}\ \text{N}}{6\pi(0.9\ \text{mPa} \cdot \text{s})(2\ \mu\text{m})} \approx 1 \times 10^{-6}\ \text{m/s}. \tag{S3}$$

During rearrangements, the distance traveled is typically on or below the order of interparticle distance, in microns; this estimate suggests that the time spent during a rearrangement is on the order of seconds.

## SB. Equation of motion

*Equation of motion in physical units*

In the text we tailor the equation of motion to the dimensionless $D_{\min}$ coordinate we wish to analyze. We present here an alternative derivation of Eq. 2, keeping physical units where possible.

The force balance for overdamped motion in a 1D potential can be written as

$$\eta \frac{dx}{dt} = -\frac{dU}{dx} + F_{\text{drive}}(t) \tag{S4}$$

for a particle with position $x$, damping coefficient $\eta$, in a potential $V(x)$ and driven by external force $F_{\text{drive}}$. A generic bistable potential can be written as a quartic function

$$U(x) = A(x - x_b)^4 - B(x - x_b)^2 + F_P(x - x_b) \tag{S5}$$

where $A$, $B$, $x_b$ and $F_P$ are parameters of the potential.

We now translate the model to our system with coordinate variable $D_{\min}$ and driving function $\gamma(t)$. Let $x = a_0 D_{\min}$ where $a_0$ is the $D^2_{\min}$ length scale. Let $F_D\gamma(t)$ be a forcing term assumed to be proportional to shear strain, with a proportionality constant $F_D$ (in force units) left to be determined. We write the equation of motion for $D_{\min}$ as

$$\eta a_0 \frac{dD_{\min}}{dt} = -\frac{dV(a_0 D_{\min})}{d(a_0 D_{\min})} + F_D\gamma(t). \tag{S6}$$

This can be rewritten as

$$\hat{\eta} \frac{dD_{\min}}{dt} = -\frac{d\hat{U}(D_{\min})}{dD_{\min}} + \gamma(t). \tag{S7}$$

where $\hat{\eta} = \eta a_0/F_D$ is a dissipation timescale, and $\hat{V}(D_{\min}) = V(a_0 D_{\min})/(a_0 F_D)$ is the dimensionless potential energy expressed in terms of $D_{\min}$. We thus arrive at Eq. 2 as defined in the main text.

*Fitting Parameters*

We then determine $\hat{\eta}$, which is not generally known *a priori* for each rearrangement. Since Eq. 2 only depends on $D_{\min}$, a 1D coordinate, there must be

$$\oint_{\text{Cycle}_i} \left(\gamma - \hat{\eta}\frac{dD_{\min}}{dt}\right) dD_{\min} = 0 \tag{S8}$$

for each driving cycle if the solution is periodic. We determined the optimal scalar $\hat{\eta}^*$ that best minimizes LHS of Eq. S8, for all cycles:

$$\hat{\eta}^* = \arg\min_{\hat{\eta}} \left| \sum_{i=1}^{18} \oint_{\text{Cycle}_i} \left(\gamma - \hat{\eta}\frac{dD_{\min}}{dt}\right) dD_{\min} \right|. \tag{S9}$$

This allows the collapse of data onto the force curve $-\hat{F}_{\text{rep}}(D_{\min})$ (defined in the main text).

The cubic parameters $\hat{A}$, $\hat{B}$, $\hat{F}_P$ and $\hat{x}_b$ (see Eq. 3 of the main text) are determined using least-squares methods on the experimental $\hat{F}_{\text{rep}}$ curves.

For the individual rearrangements shown in the main text (in their order of appearance in Sec. III), we calculated best-fit parameters $\{\hat{\eta}, \hat{A}, \hat{B}, \hat{F}_P, \hat{x}_b\}$ as defined in Eqs. 2–3, which we list in Table SI.

*Piecewise driving in numerical solutions*

A typical driving cycle consists of a sinusoidal part and a static wait period, represented as

$$\text{Oscillatory drive: } \gamma(t) = \frac{\gamma_{\max}}{2}(1 - \cos(2\pi f_i t)), \qquad t_i \le t < t_i + f_i^{-1} \tag{S10a}$$

$$\text{Recovery: } \gamma(t) = 0, \qquad t_i + f_i^{-1} \le t < t_i + f_i^{-1} + t_{\text{w}} \tag{S10b}$$

| Particle ID | $\hat{\eta}$ (s) | $\hat{A}$ | $\hat{B}$ | $\hat{F}_P$ | $\hat{x}_b$ |
|---|---|---|---|---|---|
| 3039 | 0.484 | 14.8 | 0.0890 | 0.0180 | 0.132 |
| 10956 | 0.520 | 5.63 | -0.0123 | 0.0384 | 0.183 |
| 10355 | 0.877 | 18.0 | 0.234 | 0.0373 | 0.165 |

Table SI: Model parameters used for rearrangements corresponding to Fig. 3, 4 and 5, respectively, which are used as input for eqn. (3). See main text for determination of the parameters.

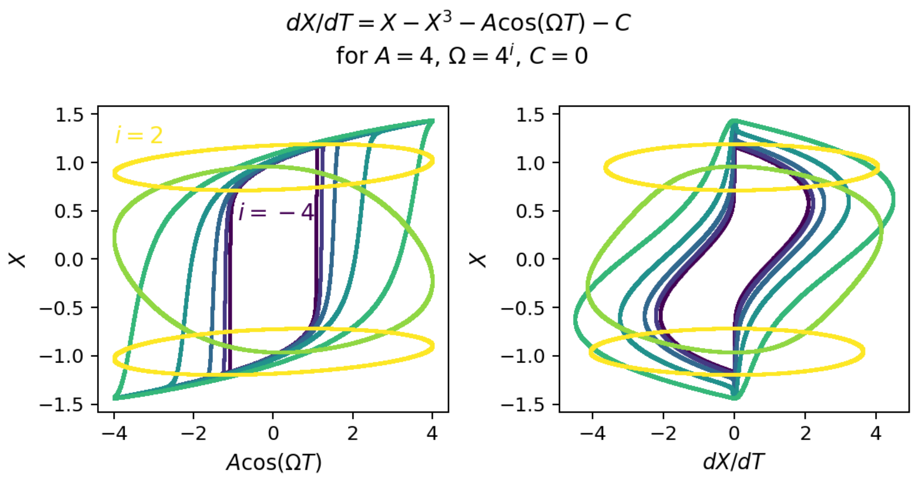


Figure S3: Family of steady state solutions of Eq. 6 for $A = 4$ and $C = 0$. Note that the stable orbit bifurcates for $\Omega > 4$.

where $f_i$ is the frequency used in the $i$th cycle, and $t_i$ is the start time of each cycle. $t_\mathrm{w}$ is the waiting period defined in the main text.

We now write down the equation of motion using Eq. 2 (see main text), using Eq. S10 as input:

$$\text{Oscillatory drive: } \frac{d\tilde{x}}{d\tilde{t}} = \sqrt{\frac{27}{4}}\left(\tilde{x} - \tilde{x}^3\right) + \frac{\gamma_{\max}}{2\hat{F}_0}\left(1 - \cos\left(2\pi f_i \tau_0 \tilde{t}\right)\right) + \hat{F}_P, \quad t_i \le \tilde{t}\tau_0 < t_i + f_i^{-1} \tag{S11a}$$

$$\text{Recovery: } \frac{d\tilde{x}}{d\tilde{t}} = \sqrt{\frac{27}{4}}\left(\tilde{x} - \tilde{x}^3\right) + \hat{F}_P, \quad t_i + f_i^{-1} \le t\tau_0 < t_i + f_i^{-1} + t_\mathrm{w}. \tag{S11b}$$

where we defined $\tilde{x} = (D_{\min} - \hat{x}_b)/\hat{x}_0$, $\tilde{t} = t/\tau_0$. Initial conditions for each piecewise segment is set such that continuity is ensured at each boundary.

## SC. Numerical results on the equation $dX/dT = X - X^3 - A\cos(\Omega T) - C$

In this section, we show details and additional results from the solutions of Eq. 6 from the main text.

A typical example using $A = 4$, $\Omega \in \{4^{-3}, 4^{-2}, \ldots, 4^2\}$, and $C = 0$ is shown in Fig. S3. Two types of behaviors are noticeable. For low $\Omega$, the loop is hysteretic and is symmetric about $X = 0$; it eventually approaches the quasi-static curve for $\Omega$ approaching 0. Here, the limits of stability are located at $(\pm 1, \mp 1/\sqrt{3})$ in the $(A\cos(\Omega T), X)$ coordinates. For $\Omega$ above some critical value between 4 and 16, the limit cycle bifurcates into two branches, each orbiting a potential minima ($X = \pm 1$).

The main result in Fig. 6 is the diagram of skipping criterion. In Fig. S4 we show several slices of the 3D equilibrium surface (once more keeping to the upper branch) along grid lines of constant $A$ and

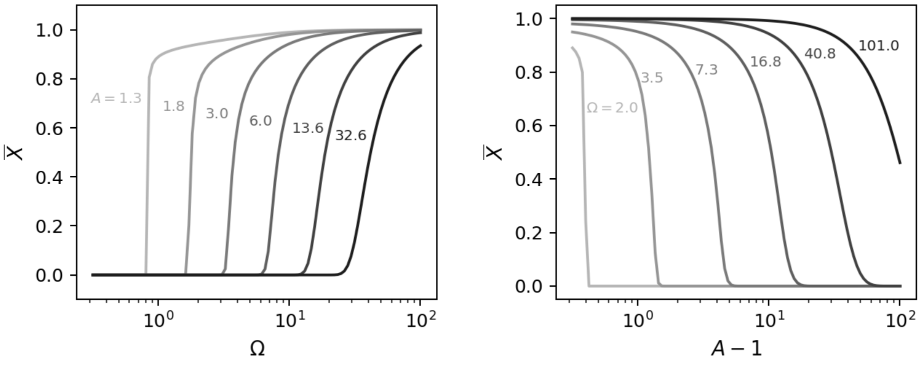


Figure S4: Switching behavior of Eq. 6 as a function of $A$ and $\Omega$ with $C = 0$. The order parameter $\bar{X}$ undergoes a pitchfork bifurcation through the line $\Omega \sim A - 1$; for clarity we only show the positive branch, while the lower branch is symmetric.

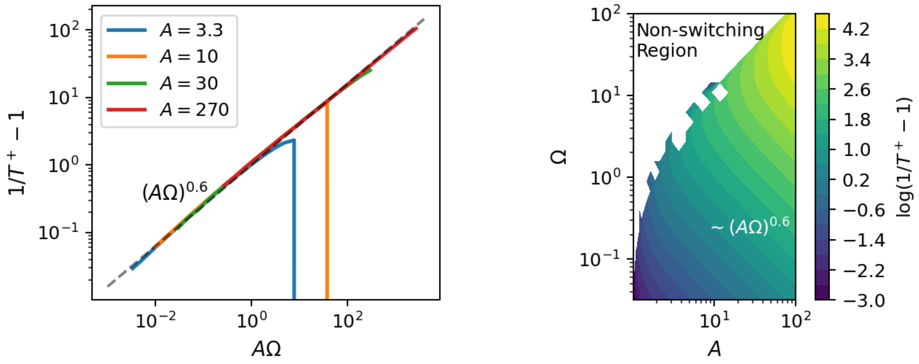


Figure S5: $1/T^+$ scaling with different parameters. In the switching regime, it follows an empirical relation $1/T^+ = 1 + (A\Omega)^{0.6}$.

$\Omega$. Spacing between data points is 10/3 times finer than Fig. 6, showing the sharp transition at small $A - 1$ and $\Omega$ values.

We are also interested in how the timescale depends on driving parameters. The timescale should be proportional to $\Delta X/(dX/dT)$, where $\Delta X$ is some characteristic length scale. In a switching event $\Delta X$ is on the order of unity. We introduce the timescale $T^+$, such that

$$\frac{1}{T^+} = \frac{dX}{dT}\bigg|_{X=0,\, dX/dT>0} \tag{S12}$$

We chose to evaluate $dX/dT$ at $X = 0$ because the definition is clear, even though it does not represent the largest $dX/dT$ value during a cycle (see Fig. S4). Note that $T^+$ is undefined for bifurcated orbits that do not pass through $X = 0$. In the $\Omega \to 0$ limit, $1/T^+$ approaches 1. In Fig. S5, we plot $1/T^+ - 1$ with $A$ and $\Omega$ parameters, keeping $C = 0$ unchanged.

We found that the quantity $A\Omega$ collapses our numerical $T^+$ curves onto a power law expression, with exponent 0.6. This scaling holds in most parts of the rearranging regime, except when approaching the phase boundary at $\Omega \approx A$ where a boundary layer develops. This suggests the results from main text is general; $A\Omega$ can be though of as the rate of change of external driving, with $\frac{d}{dT} A\cos(\Omega T) = A\Omega \sin(\Omega T)$; the sine term is approximately $\sqrt{1 - 1/A^2}$ during the transition, which is close to 1 when $A^2 \ll 1$ (less than 5% off for the smallest value, $A = 3.3$, in Fig. S5). We relate this observation to the main text via

$$A\Omega = \frac{\gamma_{\max}}{2\hat{F}_0} \cdot (2\pi f \tau_0) \tag{S13}$$

using definitions in the derivation of Eq. 6 and Eq. S11; setting $A\Omega = 1$ gives the timescale $\tau_C$.
